# Supplementary material for: Purcell enhancement of erbium ions in TiO$_{2}$ on silicon nanocavities
Source: arXiv:2204.09859 source file (2022-04-21)
Supplement: Supplementary file 1 [file 20220418_submission_Purcell_enhancement_of_erbium_ions_in_TiO2_on_silicon_nanocavities_SI.pdf]

Supplementary Information for

**Purcell enhancement of erbium ions in TiO<sub>2</sub> on silicon  
nanocavities**

Alan M. Dibos,<sup>\*,†,‡</sup> Michael T. Solomon,<sup>¶,§,‡</sup> Sean E. Sullivan,<sup>§,‡</sup> Manish K. Singh,<sup>¶,§</sup>  
Kathryn E. Sautter,<sup>§,¶</sup> Connor P. Horn,<sup>¶,§</sup> Gregory D. Grant,<sup>¶,§</sup> Yulin Lin,<sup>†</sup> Jianguo Wen,<sup>†</sup>  
F. Joseph Heremans,<sup>§,‡,¶</sup> Supratik Guha,<sup>¶,¶,§</sup> and David D. Awschalom<sup>¶,§,‡</sup>

<sup>†</sup>*Nanoscience and Technology Division, Argonne National Laboratory, Lemont, IL 60439*

<sup>‡</sup>*Center for Molecular Engineering, Argonne National Laboratory, Lemont, IL 60439*

<sup>¶</sup>*Pritzker School of Molecular Engineering, University of Chicago, Chicago, IL 60637*

<sup>§</sup>*Materials Science Division, Argonne National Laboratory, Lemont, IL 60439*

E-mail: [adibos@anl.gov](mailto:adibos@anl.gov)

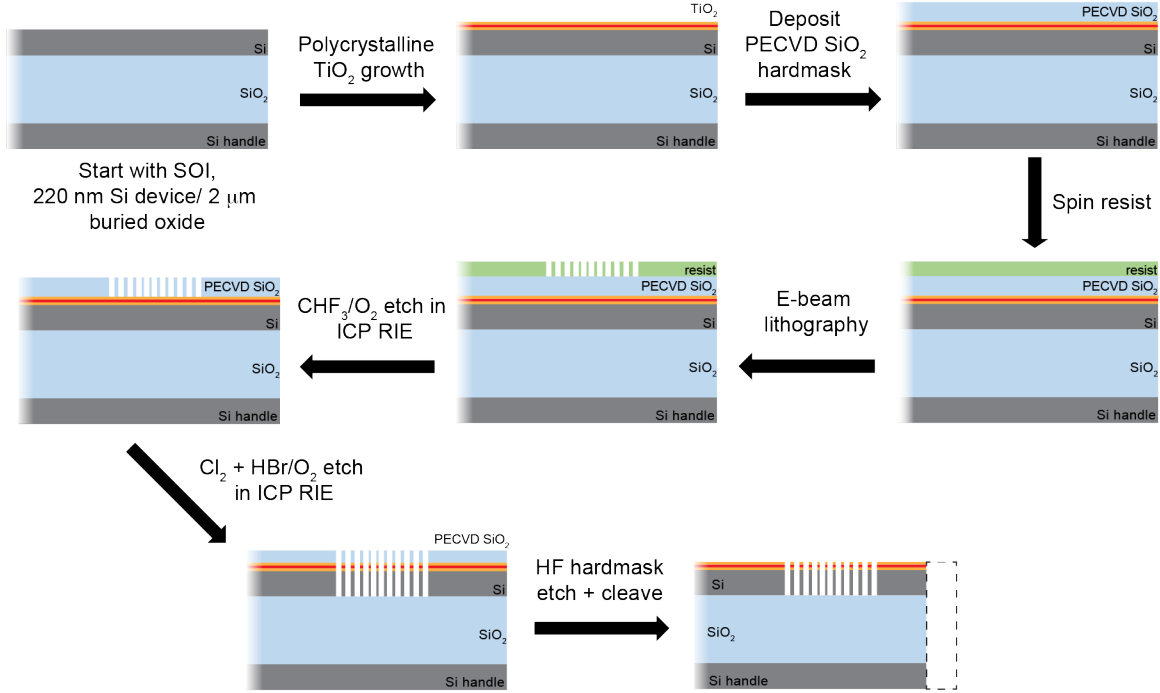

**Figure S1: Fabrication flow.** The fabrication flow used to generate 1D photonic crystal cavities from  $\text{TiO}_2$  grown atop silicon-on-insulator (SOI) wafers. Note that the various layer thicknesses are not to scale.

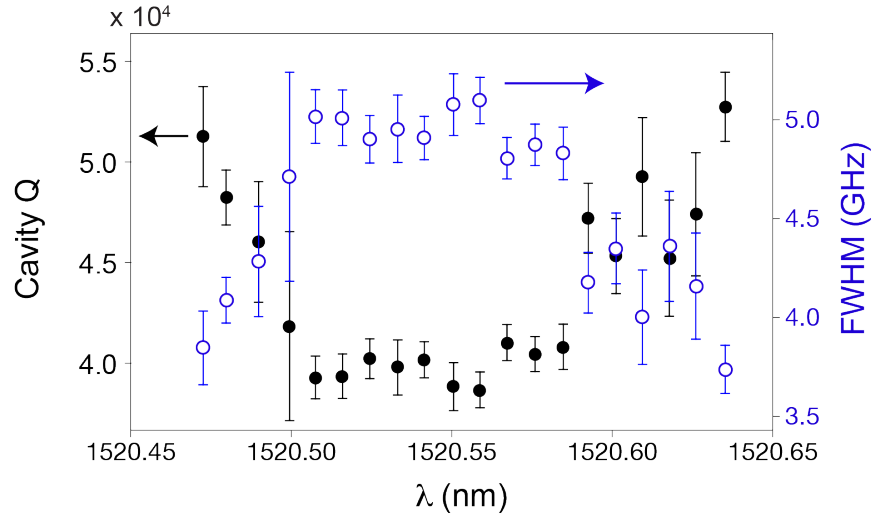

**Figure S2: Reduction in cavity quality factor near Er transition in rutile  $\text{TiO}_2$**  A plot of the cavity quality factor (Q) at  $T = 3.1$  K as measured by resonant laser reflection scan (left axis) as the cavity is systematically redshifted through the Er: rutile  $\text{TiO}_2$  transition at 1520.56 nm. The associated cavity linewidth (FWHM in GHz, right axis) as the cavity is detuned is also shown. There is a modest reduction in quality factor of  $\sim 20\%$  that recovers on the other side of the resonance, strongly suggesting that the decrease in Q is due to parasitic absorption from the relatively high spectral density of the Er ensemble in this range. This further corroborates that the decrease in the ensemble decay rate (as a function of the cavity-laser detuning when the laser is fixed at 1520.56 nm) shown Fig. 3c of the main text, is due to the presence of the cavity.
